# Supplementary material for: Cubic magneto-optic Kerr effect in Ni(111) thin films with and without twinning
Source: arXiv:2205.08298 ancillary file (2024-03-19)
Supplement: Supplementary file 1 [file CMOKE_Ni_111__PRL_Supplemental_materials.pdf]

# Supplemental Materials
# Cubic magneto-optic Kerr effect in Ni(111) thin films with and without twinning

Maik Gaerner,[1,*] Robin Silber,[2,3,*] Tobias Peters,[1] Jaroslav Hamrle,[4] and Timo Kuschel[1,†]

[1]*Center for Spinelectronic Materials and Devices, Department of Physics, Bielefeld University, Bielefeld 33615, Germany*
[2]*IT4Innovations, VŠB-Technical University of Ostrava, Ostrava 70800, Czech Republic*
[3]*Nanotechnology Centre, VŠB-Technical University of Ostrava, Ostrava 70800, Czech Republic*
[4]*Faculty of Mathematics and Physics, Charles University, Prague 12116 , Czech Republic*

## H TENSOR FOR CUBIC CRYSTAL STRUCTURES

The following derivation of the $\boldsymbol{H}$ tensor is based on the approach used in Ref. [1] in which the magneto-optic (MO) tensors of first and second order in magnetization $\boldsymbol{M}$ are derived. The coordinate system and sign conventions used in this work are described in Ref. [2]. The cartesian $\hat{x}$, $\hat{y}$, $\hat{z}$ system, describing the sample orientation, is right-handed. The $\hat{z}$-axis is normal to the sample surface and points into the sample. The $\hat{y}$-axis is parallel to the plane of incident light and to the sample surface. Its positive direction is defined using the y-component of the wave vector of the light. We assume that the MO tensor of third order in $\boldsymbol{M}$ is a tensor of fifth rank with elements $H_{ijklm}$, such that

$$\varepsilon_{ij}^{(3)} = H_{ijklm} M_k M_l M_m \tag{S 1}$$

with $\varepsilon_{ij}^{(3)}$ being the third-order contribution of the permittivity tensor and $M_{k/l/m}$ are the components of the normalized magnetization

$$\boldsymbol{M} = \begin{bmatrix} M_1 \\ M_2 \\ M_3 \end{bmatrix} = \begin{bmatrix} M_x \\ M_y \\ M_z \end{bmatrix} = \begin{bmatrix} M_T \\ M_L \\ M_P \end{bmatrix} . \tag{S 2}$$

Upon considering the Onsager relation $\varepsilon_{ij}(\omega, \boldsymbol{M}) = \varepsilon_{ji}(\omega, -\boldsymbol{M})$, we conclude that

$$H_{iiklm} = 0 \ , \tag{S 3}$$

$$\begin{gathered} H_{ijklm} = H_{ijkml} = H_{ijlkm} = H_{ijlmk} = H_{ijmkl} = H_{ijmlk} \\ = \\ -H_{jiklm} = -H_{jikml} = -H_{jilkm} = -H_{jilmk} = -H_{jimkl} = -H_{jimlk} \ . \end{gathered} \tag{S 4}$$

Under consideration of the symmetry arguments of cubic crystal structures (crystal classes 432, $\bar{4}3m$ and $m3m$), the non-zero elements of the permittivity of third order in $\boldsymbol{M}$ using the Voigt notation write

$$\begin{bmatrix} \varepsilon_{23}^{(3)} \\ \varepsilon_{31}^{(3)} \\ \varepsilon_{12}^{(3)} \\ \varepsilon_{32}^{(3)} \\ \varepsilon_{13}^{(3)} \\ \varepsilon_{21}^{(3)} \end{bmatrix} = \begin{bmatrix} H_{123} & 0 & 0 & 0 & 0 & 3H_{125} & 0 & 3H_{125} & 0 & 0 \\ 0 & H_{123} & 0 & 3H_{125} & 0 & 0 & 0 & 0 & 3H_{125} & 0 \\ 0 & 0 & H_{123} & 0 & 3H_{125} & 0 & 3H_{125} & 0 & 0 & 0 \\ -H_{123} & 0 & 0 & 0 & 0 & -3H_{125} & 0 & -3H_{125} & 0 & 0 \\ 0 & -H_{123} & 0 & -3H_{125} & 0 & 0 & 0 & 0 & -3H_{125} & 0 \\ 0 & 0 & -H_{123} & 0 & -3H_{125} & 0 & -3H_{125} & 0 & 0 & 0 \end{bmatrix} \begin{bmatrix} M_1^3 \\ M_2^3 \\ M_3^3 \\ M_2 M_3^2 \\ M_3 M_1^2 \\ M_1 M_2^2 \\ M_3 M_2^2 \\ M_1 M_3^2 \\ M_2 M_1^2 \\ M_1 M_2 M_3 \end{bmatrix} . \tag{S 5}$$

## PERMITTIVITY TENSOR FOR (111)-ORIENTED CUBIC CRYSTAL STRUCTURES

The elements of the rotated tensors $\boldsymbol{G}^{(111)}$ and $\boldsymbol{H}^{(111)}$ are calculated using

$$\begin{gathered} G_{ijkl}^{(111)} = a_{in} a_{jo} a_{kp} a_{lq} G_{nopq}^{(001)} \ , \\ H_{ijklm}^{(111)} = a_{in} a_{jo} a_{kp} a_{lq} a_{mr} H_{nopqr}^{(001)} \ , \end{gathered} \tag{S 6}$$

with $G^{(001)}_{nopq}$ and $H^{(001)}_{nopqr}$ being the elements of the initial tensors $\boldsymbol{G}^{(001)}$ and $\boldsymbol{H}^{(001)}$. Moreover, $a_{\nu\omega}$ ($\nu, \omega = x, y, z$) are elements of the 3x3 matrix $\boldsymbol{a}$ which is the product of the three rotation matrices representing rotations around the $x$-, $y$- and $z$-axis of the coordinate system. Note that in case of cubic crystal structures, $\boldsymbol{\varepsilon}^{(0)}$ and $\boldsymbol{K}$ are isotropic and therefore not affected by the rotations [1].
The off-diagonal elements of the permittivity tensor up to third order in $\boldsymbol{M}$ of a (111)-oriented cubic crystal then write

$$\begin{aligned}\varepsilon^{(111)}_{yx/xy} = &\left(2G_{44} + \frac{1}{3}\Delta G\right) M_L M_T \mp \frac{1}{3\sqrt{2}}\Delta H \sin(3\alpha) M_L^3 \pm \frac{1}{3\sqrt{2}}\Delta H \cos(3\alpha) M_T^3 \\ &\mp \frac{1}{\sqrt{2}}\Delta H \cos(3\alpha) M_T M_L^2 \pm \frac{1}{\sqrt{2}}\Delta H \sin(3\alpha) M_L M_T^2 \ ,\end{aligned} \tag{S 7}$$

$$\begin{aligned}\varepsilon^{(111)}_{zx/xz} = &\pm K M_L - \frac{2}{3\sqrt{2}}\Delta G \sin(3\alpha) M_L M_T - \frac{1}{3\sqrt{2}}\Delta G \cos(3\alpha)(M_T^2 - M_L^2) \\ &\pm \frac{1}{2}(H_{123} + H_{125}) M_L^3 \pm \frac{1}{2}(H_{123} + 3H_{125}) M_L M_T^2 \ ,\end{aligned} \tag{S 8}$$

$$\begin{aligned}\varepsilon^{(111)}_{yz/zy} = &\pm K M_T + \frac{2}{3\sqrt{2}}\Delta G \cos(3\alpha) M_L M_T - \frac{1}{3\sqrt{2}}\Delta G \sin(3\alpha)(M_T^2 - M_L^2) \\ &\pm \frac{1}{2}(H_{123} + H_{125}) M_T^3 \pm \frac{1}{2}(H_{123} + 3H_{125}) M_T M_L^2 \ ,\end{aligned} \tag{S 9}$$

in case of a pure in-plane magnetization ($M_P = 0$). Using these elements, the analytical equation for the Kerr angles with $s$- and $p$-polarized light is derived by inserting Eqs. (S 7)-(S 9) into Eqs. (1) and (2) of the main text. This analytical equation is

$$\begin{aligned}\Phi^{(111)}_{s/p} = &\pm A_{s/p}\Bigg[\left(2G_{44} + \frac{1}{3}\Delta G - \frac{K^2}{\varepsilon_d}\right) M_L M_T \\ &\mp \frac{1}{3\sqrt{2}}\left(\Delta H + \frac{K\Delta G}{\varepsilon_d}\right)\sin(3\alpha) M_L^3 \pm \frac{1}{3\sqrt{2}}\left(\Delta H + \frac{K\Delta G}{\varepsilon_d}\right)\cos(3\alpha) M_T^3 \\ &\mp \frac{1}{\sqrt{2}}\left(\Delta H + \frac{K\Delta G}{\varepsilon_d}\right)\cos(3\alpha) M_T M_L^2 \pm \frac{1}{\sqrt{2}}\left(\Delta H + \frac{K\Delta G}{\varepsilon_d}\right)\sin(3\alpha) M_L M_T^2\Bigg] \\ &+ B_{s/p}\Bigg[\pm K M_L \pm \frac{1}{2}(H_{123} + 3H_{125}) M_L^3 \pm \frac{1}{2}(H_{123} + 3H_{125}) M_L M_T^2 \\ &- \frac{2}{3\sqrt{2}}\Delta G \sin(3\alpha) M_L M_T - \frac{1}{3\sqrt{2}}\Delta G \cos(3\alpha)(M_T^2 - M_L^2)\Bigg] \ .\end{aligned} \tag{S 10}$$

$M_L$ and $M_T$ can also be expressed as

$$M_T = \cos(\mu) \ , \qquad M_L = \sin(\mu) \ . \tag{S 11}$$

Here, the angle $\mu$ describes the direction of the normalized magnetization vector. It is defined as the angle between the in-plane direction of $\boldsymbol{M}$ and the $\hat{x}$-axis of our coordinate system.

## EIGHT-DIRECTIONAL METHOD

During the eight-directional method, the MOKE signal is measured for eight different in-plane magnetization directions $\mu = 0° + k \cdot 45°, k = \{0, 1, ..., 7\}$. During the measurement process, the Kerr angles are usually measured five times for each of the eight magnetic field directions. This process is repeated in angular steps of 3° for a full sample rotation of 360°. The measured values for each sample position are then averaged and summed up and/or subtracted in order to calculate $\Phi_{M_L, M_L^3}$, $\Phi_{M_T^3}$, $\Phi_{M_L M_T}$ and $\Phi_{M_T^2 - M_L^2}$ according to Eqs. (4)-(7).
The individual eight-directional measurements of the five additional samples which are referenced in Fig. 2 in the main

text are displayed alongside the corresponding off-specular XRD scans in Fig. S 1. For the sample with 7% of twinning, the CMOKE contributions $\Phi_{M_L,M_L^3}$ and $\Phi_{M_T^3}$ have absolute amplitudes of $(1.77 \pm 0.02)$ mdeg and $(1.75 \pm 0.01)$ mdeg. For the sample with 96% of twinning, the absolute amplitudes of $\Phi_{M_L,M_L^3}$ and $\Phi_{M_T^3}$ are $(0.00 \pm 0.02)$ mdeg and $(0.03 \pm 0.02)$ mdeg.

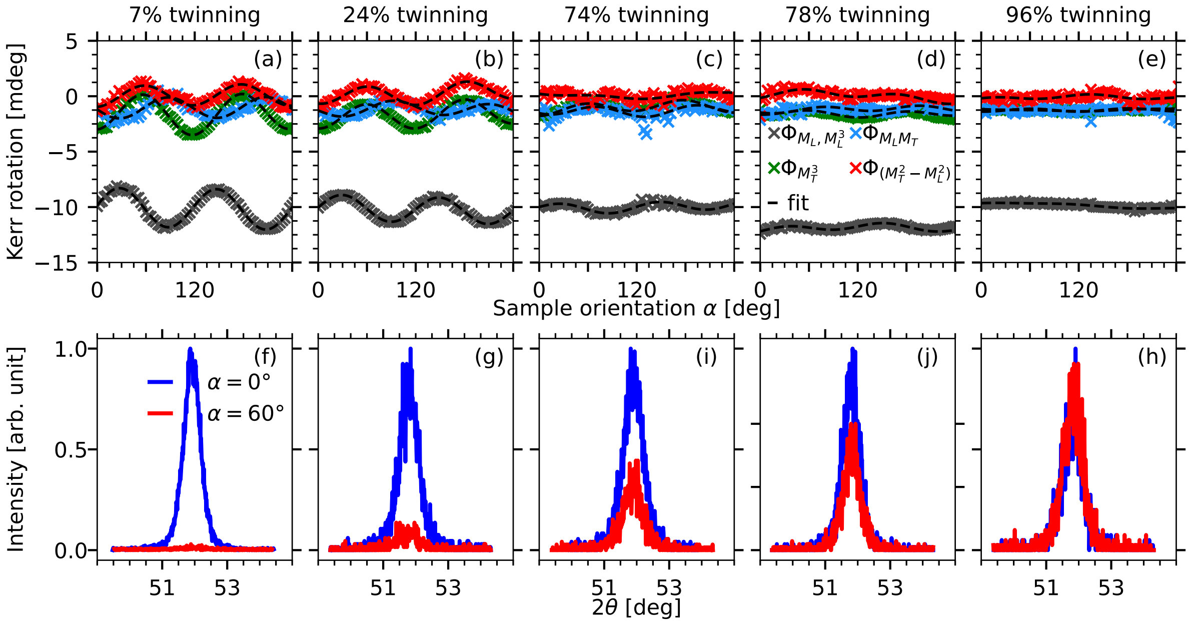


FIG. S 1. MOKE and XRD data of the additional Ni(111) samples with varying amounts of twinning. (a-e) Eight-directional method performed with a magnetic field strength of 230 mT using a wavelength of 635 nm. (f-h) Off-specular XRD scans of the Ni{200} peaks at selected $\alpha$ angles.

For sample 1 (9.8% of twinning) and sample 2 (86% of twinning) the eight-directional method was carried out for both Kerr rotation and Kerr ellipticity at two different wavelengths of $\lambda$=406 nm and $\lambda$=635 nm. The measurement of the Kerr ellipticity was conducted by placing a $\lambda/4$ waveplate in the optical path between the sample and the detector. The resulting measurements are displayed in Fig. S 2. Eventhough the amplitudes of the threefold angular dependencies vary, they appear in all measurements of the Kerr rotation as well as the Kerr ellipticity and decrease in the sample with a greater amount of twinning.

As can be seen in Figs. S 2(a,b,c,e,f), $\Phi_{M_T^3}$ has a non-vanishing offset which is not described by theory. In order to exclude a possible setup misalignment as the cause of this offset, measurements with deliberately misaligned magnets have been conducted. In case that the in-plane applied magnetic field along the transverse axis possesses an out-of-plane component or a longitudinal component, an additional contribution to the $\Phi_{M_T}$ signal is generated. In order to investigate this possible influence on $\Phi_{M_T}$, additional measurements were made while the magnets have been tilted along the longitudinal and the out-of-plane axis by $\pm 1°$. However, no significant changes to the offsets have been observed.

Furthermore, a magneto-optic polar effect $\propto M_P$ (e.g. due to the miscut of the Ni layer) would change its sign upon a sample rotation of 180°. This consideration limits possible out-of-plane CMOKE contributions to those which are even in $M_P$, such as contributions $\propto M_L M_P^2$. The anisotropic CMOKE contributions which are odd in $M_P$ could not produce a constant threefold angular dependence since they would change their sign when the sample is rotated by 180°. Upon further consideration of the structural sample properties, it becomes evident that no $M_P$ component should be induced by the miscut when its step edges are aligned parallel to $\boldsymbol{H}$. Therefore, also a contribution $\propto M_L M_P^2$ should vanish for certain sample orientations so that a threefold oscillation with constant amplitude cannot be caused by it. Thus it is unlikely that the observed, additional CMOKE contribution is due to an $M_P$ component.

## MAGNETIC ANISOTROPY

In order to show that the threefold angular dependence of $\Phi_{M_L,M_L^3}$ and $\Phi_{M_T^3}$ actually stems from CMOKE and is not due to magnetic anisotropy, we present measurements of the coercive field and remanent magnetization depending on

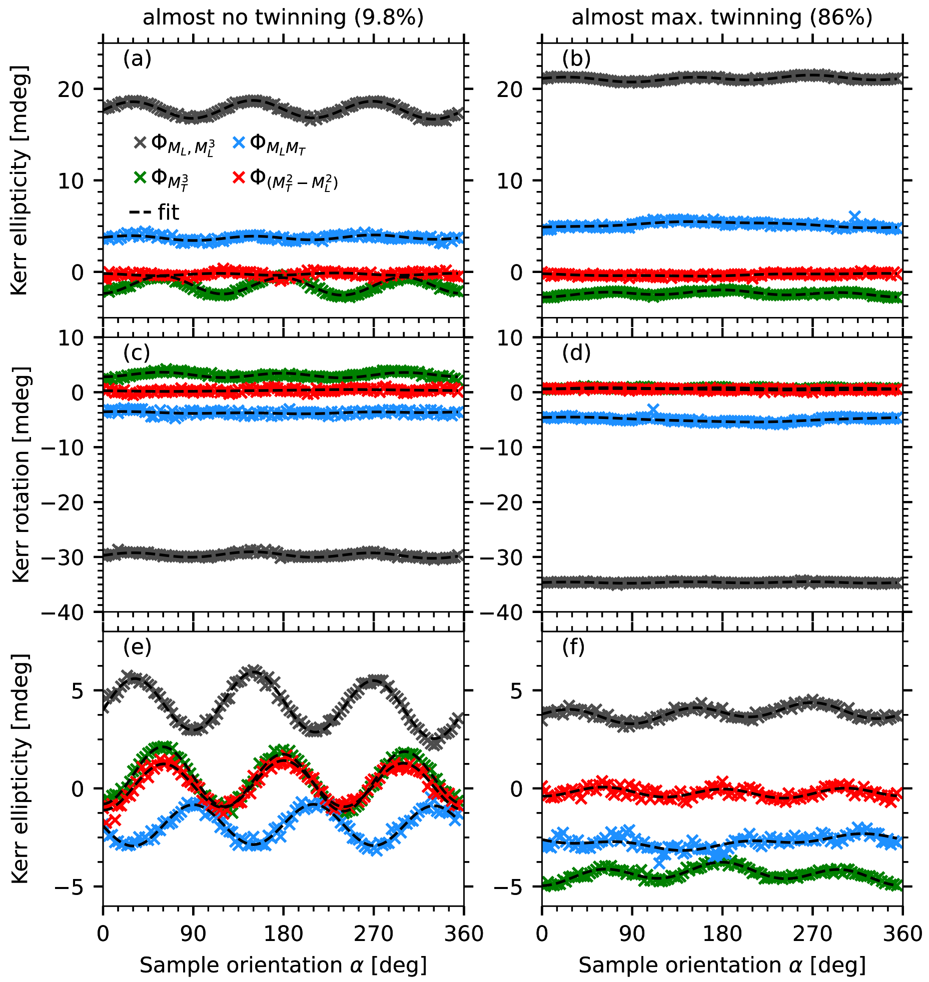


FIG. S 2. Eight-directional method performed for samples 1 (left) and 2 (right) with a magnetic field strength of 230 mT. (a,b) Kerr ellipticity using a wavelength of $\lambda$=635 nm. (c,d) Kerr rotation using $\lambda$=406 nm. (e,f) Kerr ellipticity using $\lambda$=406 nm.

the orientation of sample 1. As displayed in Fig. S 3, the sample mainly possesses a uniaxial magnetic anisotropy with a magnetic easy axis along $\alpha \approx 45^\circ$ and $\alpha \approx 225^\circ$. This means that the magnetic easy axis of sample 1 is oriented parallel to the step edges of the Ni layer. Note that this behaviour agrees with observations in Co films with vicinal interface [3]. Since the sample possesses a uniaxial magnetic anisotropy, it can be concluded that the anisotropy in the MOKE signal in magnetic saturation is due to the anisotropy of the CMOKE itself.

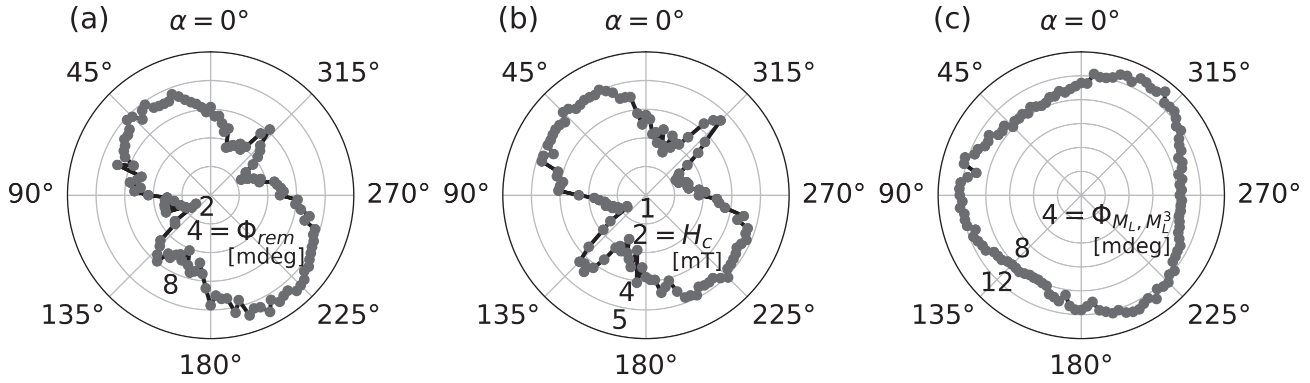


FIG. S 3. Anisotropy of (a) the magnetic remanence, (b) the coercive field and (c) the magnetically saturated $\Phi_{M_L,M_L^3}$ signal in sample 1.

## PREPARATION OF SAMPLES WITH DIFFERENT DEGREES OF TWINNING

In order to prepare Ni layers with different degrees of twinning, the substrate treatment before the thin film deposition was altered as described in the main text. In Fig. S 4 we show that both the ultrasonic treatment with Acetone, Isopropanol and Ethanol as well as the annealing time of the substrate before deposition influence the amount of twinning in the Ni layer. On the substrates which had undergone the ultrasonic treatment, the degree of twinning in the Ni layer tends to decrease with long annealing times. However, no clear monotonic dependence between the annealing time and the degree of twinning can be observed. The degree of twinning in the Ni layer is high on the substrates which had not undergone the ultrasonic treatment, even after longer annealing times.

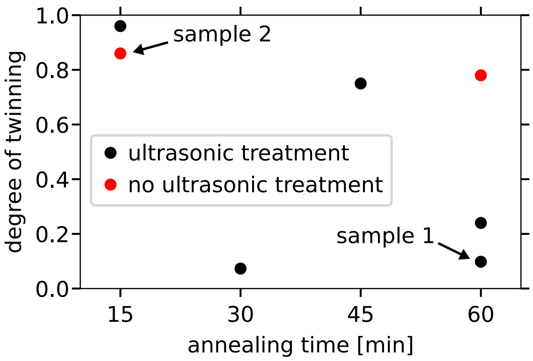


FIG. S 4. Degree of twinning of all samples plotted against the annealing time of the substrate before the deposition of the Ni layer.

## MAGNETIC FIELD DEPENDENCE

The dependencies of the amplitudes and offsets on the magnetic field strength are displayed in Fig. S 5 for sample 1 and sample 2. The contributions $\Phi_{M_L,M_L^3}$ and $\Phi_{M_T^3}$ have similar amplitudes, just as $\Phi_{M_L M_T}$ and $\Phi_{M_T^2-M_L^2}$, which is also predicted by Eqs. (4)-(7). Again, the amplitudes of all MOKE contributions (Figs. S 5(a,c)) are smaller for the twinned sample compared to the sample with almost no twinning, while the offsets of all MOKE contributions (Figs. S 5(b,d)) are independent from twinning. Only the offset of $\Phi_{M_L,M_L^3}$ deviates slightly (black data in Fig. S 5(b)) due to small differences in the Ni thicknesses. The first data points of the magnetic field dependence up to a few tens of mT belong to the magnetically unsaturated Ni layer. Here, the data deviates from the residual data progress at larger magnetic field strengths. However, when the samples are magnetically saturated, a slight decrease of the CMOKE amplitudes with increasing magnetic field (Fig. S 5(a)) and a slight increase of the QMOKE amplitudes of the non-twinned sample (Fig. S 5(c)) still remain. Most offsets do not show a dependence on the magnetic field strength if the Ni layer is saturated (Fig. S 5(b,d)). Only the $\Phi_{M_L M_T}$ offset increases slightly with increasing magnetic field strength.

## X-RAY DIFFRACTION AND REFLECTIVITY MEASUREMENTS

X-ray diffraction (XRD) $\theta - 2\theta$ scans were performed for all samples. Here, we show results for the two main samples (sample 1 and sample 2). The characteristic peaks in Figs. S 6(a,b) clearly show that the Ni layers are (111)-oriented in both samples. The thicknesses of the Ni- and capping-layers as well as the roughnesses of each interface were characterized by x-ray reflectivity (XRR). The XRR curves for samples 1 and 2 are displayed in Figs. S 6(c) and S 6(d), respectively. They were analyzed using the open-source software GENX [4] which is based on the Parratt algorithm [5]. The resulting values are displayed in Tab. S I.

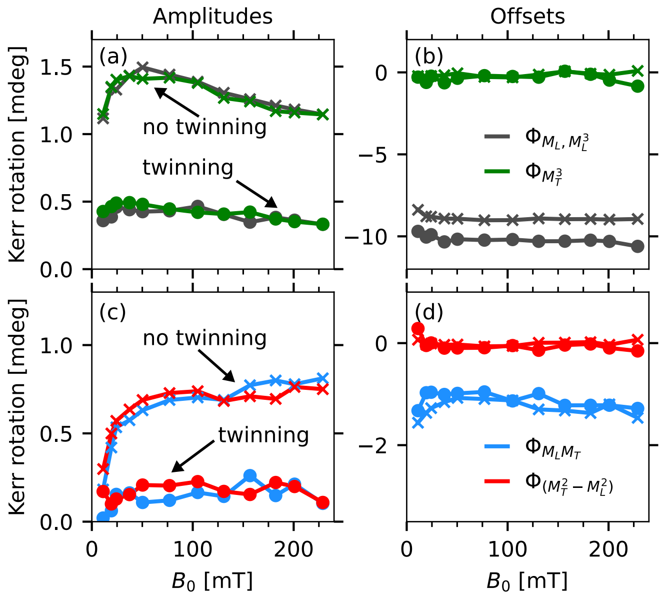


FIG. S 5. Dependence of individual MOKE contributions on the applied magnetic field for a wavelength of 635 nm. Shown are (a), (c) amplitudes and (b), (d) offsets for sample 1 (dotted data points) and sample 2 (crosses).

| Sample 1 | | | | Sample 2 | | | |
|---|---|---|---|---|---|---|---|
| Layer | $d$ [nm] | $\sigma$ [nm] | $\epsilon_d$ | Layer | $d$ [nm] | $\sigma$ [nm] | $\epsilon_d$ |
| $SiO_x$<br>Si | 3.1 | 0.0 | 3.01+0i<br>10.74+1.36i | $SiO_x$<br>Si | 3.3 | 0.6 | 2.12+0i<br>19.13+2.14i |
| Ni | 22.5 | 1.7 | -10.59+21.12i | Ni | 20.0 | 1.4 | -13.10+13.66i |
| MgO | - | 0.9 | 3.01+0i | MgO | - | 0.5 | 3.10+0i |

TABLE S I. Layer thicknesses $d$ and roughnesses $\sigma$ of samples 1 and 2, extracted via XRR fits. The thickness of the native $SiO_x$ cannot be determined separately by XRR since Si and $SiO_x$ have very similar densities. However, for the numerical simulation a $SiO_x$ thickness of 0.9 nm was estimated [2, 6]. In addition, the complex permittivities of all layers, gathered via ellipsometry at $\lambda$=635 nm, are shown.

## ONEFOLD ANGULAR DEPENDENCE

The vicinal interface sensitive magneto-optical Kerr effect (VISMOKE) can occur in ferromagnetic thin films which are deposited onto stepped substrates [7]. This VISMOKE contribution to the overall MOKE signal has a onefold angular dependence. This corresponds to the observed angular dependence in the Ni(111) samples which is predominantly visible in $\Phi_{M_L,M_L^3}$. The VISMOKE effect is maximal in $\Phi_{M_L,M_L^3}$ when the sample direction, in-plane and perpendicular to the step edges, is parallel to the incidence plane of the light [7]. This means that the vicinal direction (the direction perpendicular to the step edges) is aligned with the largest VISMOKE signal. The absolute miscut angle, which can be measured using XRD, should also be maximal when measuring along this vicinal direction. The miscut angle is determined for different sample orientations $\alpha$, by measuring XRD rocking-curves of the Ni(111) peak. Measurements of the miscut angle and $\Phi_{M_L,M_L^3}$ are displayed in Figs. S 7(a,b).

## NUMERICAL SIMULATIONS

To perform the numerical simulations, the complex permittivities $\epsilon_d$ (gathered via ellipsometry, see Tab. S I), the thicknesses of all layers in the stack (gathered via XRR and using an estimated $SiO_x$ thickness of 0.9 nm [2, 6]), the wavelength of the light and the angle of incidence used in the experiment were defined as fixed parameters in the model. The unknown MO parameters were set as free parameters. Then, the light propagation in the anisotropic multilayer structure and thus the Kerr angles for arbitrary magnetization directions were simulated using Yeh's transfer matrix formalism [8] and fitted to the experimental data. The fit of $\Phi_{M_L,M_L^3}$, $\Phi_{M_L M_T}$ and $\Phi_{M_T^2-M_L^2}$ of sample 1 using numerical simulations up to third order in $\boldsymbol{M}$ is displayed in Fig. S 8(a). The superimposed onefold angular dependency due to VISMOKE has been subtracted before the numerical fitting. The fit of the same data up

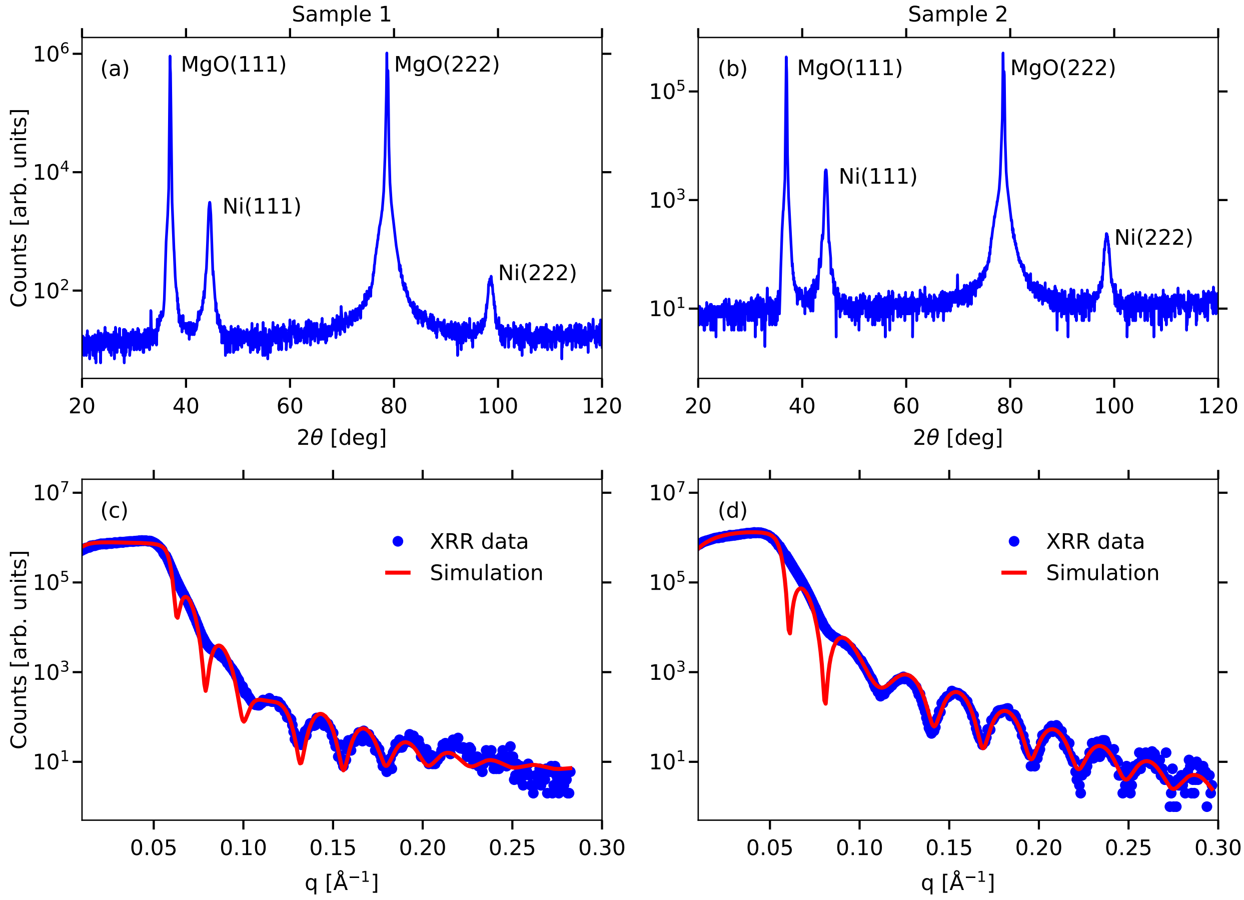


FIG. S 6. X-ray characterization. (a,b) XRD measurements of samples 1 and 2. (c,d) XRR measurements of samples 1 and 2.

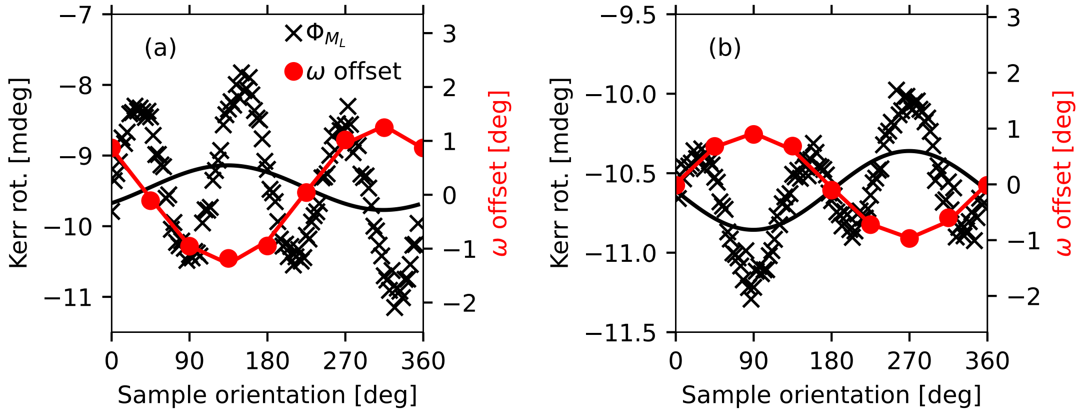


FIG. S 7. Measurements of $\Phi_{M_L,M_L^3}$ and the onefold angular dependence extracted from the fits (black lines) as well as the angular dependence of the measured miscut for (a) sample 1 and (b) sample 2.

to second order in $\boldsymbol{M}$ is shown in Fig. S 8(b). $\Phi_{M_T}$ is not shown here, since its finite offset can not be simulated. It can clearly be seen that the angular dependencies of $\Phi_{M_L,M_L^3}$ and $\Phi_{M_T^3}$ can only be fitted well if the $\boldsymbol{H}$ tensor is included in the simulations. Table S II shows the MO parameters which were used for the simulations. Note that $H_{123}$ and $H_{125}$ cannot be fitted independently and we are only fitting the anisotropy parameter of the $\boldsymbol{H}$ tensor $\Delta H = H_{123} - 3H_{125}$.

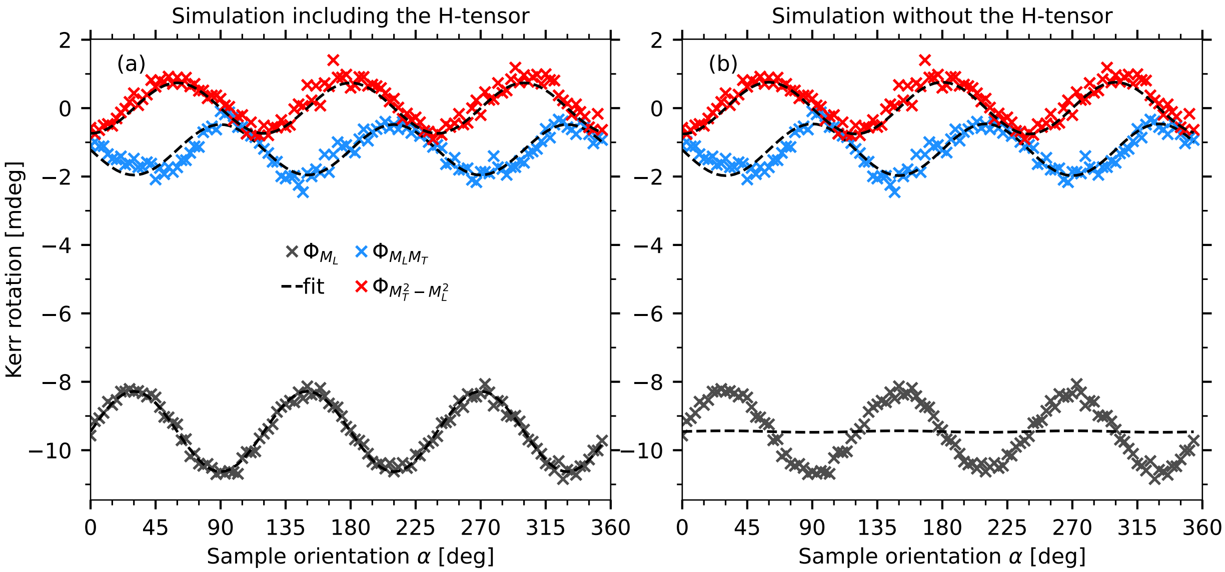


FIG. S 8. Fits of the extracted MOKE contributions of sample 1 without VISMOKE at a wavelength of 635 nm using numerical simulations including (a) permittivity described up to third order in $\boldsymbol{M}$, i.e. including the $\boldsymbol{H}$ tensor, (b) permittivity described up to second order in $\boldsymbol{M}$, i.e. without $\boldsymbol{H}$ tensor.

| MO parameter | sim. including the H-tensor | sim. without the H-tensor |
|---|---|---|
| $K$ | $-0.2419 + 0.0162i$ | $-0.2370 + 0.0170i$ |
| $G_s$ | $-0.0090 - 0.0049i$ | $-0.0085 - 0.0057i$ |
| $2G_{44}$ | $0.0045 + 0.0085i$ | $0.0042 + 0.0088i$ |
| $\Delta H$ | $0.0098 + 0.0015i$ | - |

TABLE S II. MO parameters used for the simulations in Fig. S 8.

* contributed to this work equally
† tkuschel@physik.uni-bielefeld.de

[1] Š. Višňovský, *Optics in Magnetic Multilayers and Nanostructures* (CRC Press, Boca Raton, 2006).
[2] R. Silber, O. Stejskal, L. Beran, P. Cejpek, R. Antos, T. Matalla-Wagner, J. Thien, O. Kuschel, J. Wollschläger, M. Veis, T. Kuschel, and J. Hamrle, Physical Review B **100**, 064403 (2019).
[3] A. Berger, U. Linke, and H. P. Oepen, Physical Review Letters **68**, 839 (1992).
[4] M. Björck and G. Andersson, Journal of Applied Crystallography **40**, 1174 (2007).
[5] L. G. Parratt, Physical Review **95**, 359 (1954).
[6] G. Mende, J. Finster, D. Flamm, and D. Schulze, Surface Science **128**, 169 (1983).
[7] J. Hamrle, J. Ferré, J. P. Jamet, V. Repain, G. Baudot, and S. Rousset, Physical Review B **67**, 155411 (2003).
[8] P. Yeh, Surface Science **96**, 41 (1980).
